# Supplementary material for: Capacitive coupling in hybrid Graphene-GaAs nanostructures
Source: arXiv:1503.07100 source file (2015-07-21)
Supplement: Supplementary file 1 [file Supp_Info_v3.pdf]

## Capacitive coupling in hybrid Graphene/GaAs nanostructures: Supplemental information

Pauline Simonet, Clemens Rössler, Tobias Krähenmann, Anastasia Varlet, Thomas Ihn, Klaus Ensslin, Christian Reichl, and Werner Wegscheider
*Solid State Physics Laboratory, ETH Zurich, 8093 Zurich, Switzerland*

(Dated: July 1, 2015)

# I. TI/AU REFERENCE GATES

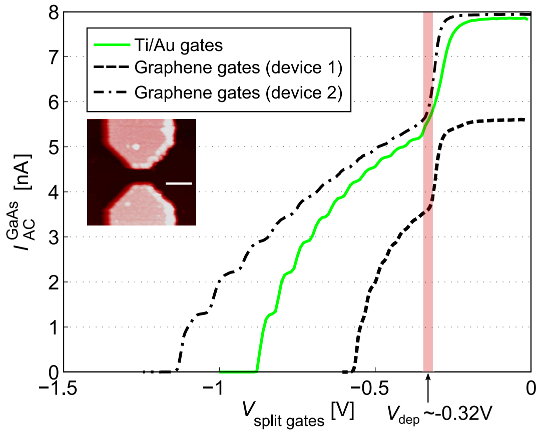


Figure S1. Current $I_{\mathrm{GaAs}}$ through the GaAs 2DEG as a function of the voltage applied to the split-gates. The red band indicates our estimation of the depletion voltage. Inset: AFM topography image of the Ti/Au split-gates. The scale bar is 500 nm.

The effect of graphene split-gates on the underlying 2DEG was compared to that of Ti/Au evaporated split-gates, whose geometry is shown in Fig. S1. The distance between the Ti/Au split-gates is 270 nm which is larger than the gap of the first device (shown in Fig. 1 of the main text) but smaller than the gap of the second (see Fig. 2 of the main text). The depletion voltage ($V_{\mathrm{dep}} \approx -0.32$V), marked by a red band in Fig. S1, is approximately the same for all devices.

# II. NON-DAMAGING ETCHING PROCESS

The graphene etching proved to be more challenging on a GaAs/AlGaAs heterostructure than on insulating substrates like $SiO_2$ or hexagonal boron nitride. Indeed, our standard procedure consisting of reactive ion etching (RIE) with an $Ar/O_2$ plasma created defects in the GaAs 2DEG below the surface.

Figure S2 illustrates the successive tests we performed to find a suitable process. A reference sample was made by evaporating Ti/Au split-gates on the GaAs/AlGaAs heterostructure in order to define six identical QPCs in the 2DEG. Three were exposed to our standard RIE step suited to etch graphene. Then, the current flowing in the 2DEG was measured as the six QPCs were alternately

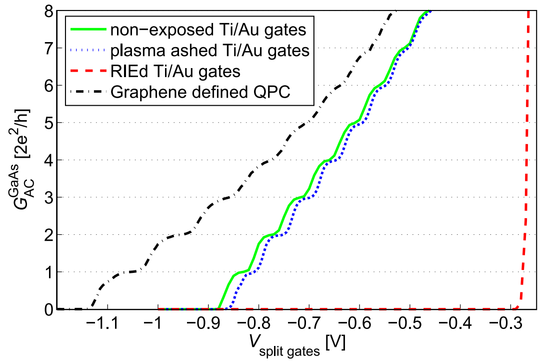


Figure S2. Conductance $G_{\mathrm{GaAs}}$ through the GaAs 2DEG as a function of the voltage applied to top split-gates. Resistances of 2.575 kΩ for the Ti/Au split-gates and of 2.530 kΩ for the graphene gates have been subtracted from the data.

pinched off. Quantized conductance was measured for the three non-exposed QPCs (green continuous curve in Fig. S2). However, as soon as the exposed split-gates depleted the 2DEG directly underneath, the current in the 2DEG dropped abruptly to zero (red dashed curve in Fig. S2). We therefore concluded that the 2DEG was damaged by the RIE exposure and does not conduct anymore.

In an RIE chamber, the sample is mainly bombarded with heavy ions such that unprotected carbon atoms are sputtered away[1]. These high-energy incident ions might get implanted in the GaAs/AlGaAs heterostructure and result in the suppressed conductance.

A less damaging technique to etch graphene is thus needed to fabricate hybrid nanostructures. Plasma ashing is a more chemical and undirected etching process relying on the oxidation of graphene by a high pressure gas of oxygen radicals[1]. The same test with the remaining three intact Ti/Au split-gates revealed that plasma ashing did not induce any significant change to the QPC transport (compare the continuous green line with the blue dotted line in Fig. S2). But this softer technique is also less efficient to etch through resist residues that remain on the graphene flake after contact deposition and chemical cleaning. Also, annealing at 300 °C in a $Ar/H_2$ gas flow led to a leakage between the gold topgates and the 2DEG (presumably due to the diffusion of gold through the heterostructure). We therefore used an alternative technique to clean graphene. Following Goossens *et al.*[2], we mechanically cleaned graphene using an AFM tip in contact mode while controlling the force applied on the flake. The area around the gold split-gates

used for the plasma ashing test were also AFM-cleaned before the ashing step.
Hence, the devices shown in the main text were defined by plasma ashing into two split-gates for the first device and into a graphene ribbon with side-gates for the second. The stepwise decrease of the GaAs conductance for the second device is shown as the black dashed-dotted line in Fig. S2.

## III. CHARGE DETECTION IN OUR SYSTEM

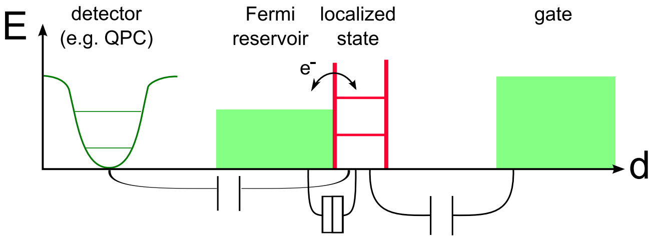


Figure S3. Energy-distance diagram of a localized state (the charge trap in our system) capacitively coupled to a gate and to a detector, and tunnel-coupled to a Fermi reservoir.

Charge detection was pioneered by Field et al.[3] in 1993. A charge detector can be any system whose conductance depends strongly on its electrostatic potential. The most well-known charge detectors are QPCs and quantum dots, but the strong conductance fluctuations of graphene nanostructures, observed as a function of gate voltages, also make them suitable detectors. The detection process can be conceptually split in two steps: a change of occupation in a charge trap induces a small effective change in the potential of a nearby detector, because of the Coulomb interaction between the two. This effective change in potential induces a change in the detector's conductance, depending on its sensitivity. If this conductance variation is measurable, the charge can be detected.

In our system, the electric field from individual charge carriers added to the graphene ribbon are strongly screened by the electronic gas in the nanoribbon itself, which explains why such a carrier cannot be detected by the QPC in the GaAs. If the ribbon could be tuned into the Coulomb blockade regime, which typically arises close to the charge neutrality point, then intra-ribbon screening would be strongly reduced and charge detection would be possible.

However, when a charge trap is loaded with a charge carrier, it induces an electrostatic potential in both the graphene ribbon and the 2DEG's QPC. This will result in kinks in their respective conductances, as seen in Fig. S4 where a cut from Fig. 3(b) and 3(c) (main text) at $V_{GR} = 60\,\mathrm{mV}$ is shown.

Kinks in the graphene conductance in Fig. S4(c) are very pronounced, but corresponding kinks in the QPC

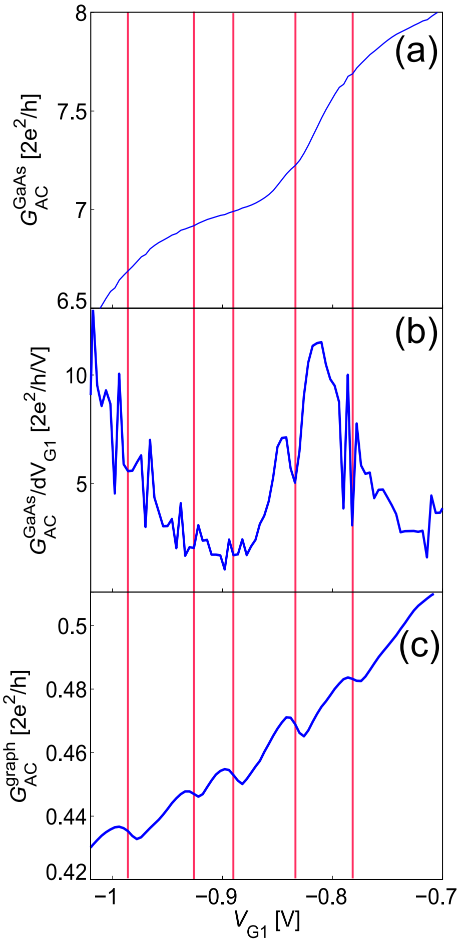


Figure S4. QPC conductance (a), QPC transconductance (b) and graphene ribbon's conductance (c) for $V_{GR} = 60\,\mathrm{mV}$, $V_{G2} = -500\,\mathrm{mV}$. (b) and (c) corresponds to cuts from Fig. 3(b) and 3(c) in the main text. Kinks reproduced in the different conductances are marked with red lines.

conductance (a) are barely seen. They are better visible as dips in the QPC transconductance (b). As expected, the sensitivity of the GaAs QPC is larger when its transconductance is larger (for $V_{G1} > -0.85\,\mathrm{V}$). The fact that the detection signal is larger in the graphene ribbon than in the GaAs QPC again indicates that charge traps are better coupled (i.e. probably spatially closer) to the graphene structure. The QPC curves suffer from noise and show other kinks unrelated to the charges detected by the ribbon - it probably detects other defects in the heterostructure. Thus, it is difficult to identify corresponding charge traps in both detectors on the basis of single curves. The maps presented in the main text however show that the kinks in the graphene conductance and corresponding dips in the QPC transconductance do occur at the same positions for a large range of voltages and confirm that the same charges are detected by both the graphene ribbon and the GaAs QPC.

The kinks in the graphene conductance can be monitored as a function of the two graphene side-gates volt-

ages $V_{G1}$ and $V_{G2}$ (not shown). The slopes of these kinks indicate that there are two groups of charge traps: one group closer to $G_1$ and another closer to $G_2$. However, this does not give any information about the depth of those charge traps. They could in principle be in the doping layer at $z = 45\,\text{nm}$. The argument developed in the next section shows that they are most probably in the same plane as the graphene structure.

## IV. TUNNEL-COUPLED CHARGE TRAPS

Maps of conductance resonances in graphene nanoribbons measured in the parameter plane of two gate voltages are found in the literature[4,5]. The observed resonances in these cases originate in localized states in the graphene ribbon. In these maps, the lines along which the resonance positions are tuned have negative slopes. This reflects the fact that a more positive voltage on one gate can be compensated by a more negative voltage on the other gate. It implies that the localized states are populated via a third reservoir serving as a reference for the gate voltages (see Fig.S3), i.e. the graphene ribbon.

In contrast, the kinks in Fig. 3(b) and (c) of our main text have positive slopes in the plane of $V_{G1}$ and $V_{GR}$. This can be explained if either $G_1$ or the ribbon acts as the reservoir from which the detected charge trap states are filled. Indeed, a charge trap tunnel-coupled to the graphene ribbon would then be depopulated by a more negative voltage on $V_{G1}$ (the gate in Fig. S3). However, in order to repopulate it, $V_{GR}$ (the Fermi reservoir in Fig. S3) also needs to be decreased, resulting in positive slopes for the lines along which such kinks are tuned in the $V_{G1}$ - $V_{GR}$ plane. The same argument applies to a charge trap tunnel-coupled to the gate $G_1$. As the slopes of the kinks in Fig. 3(b) and (c) in the main text are positive, we believe that the detected charge traps are tunnel-coupled to $G_R$ or $G_1$.

A defect in the doping layer would reside 45 nm deeper than the graphene and would very improbably be tunnel-coupled to one of the two. We therefore believe that charge traps are most likely located in the plane of the graphene structure.

## REFERENCES


[1] G. Franz, *Low Pressure Plasmas and Microstructuring Technology* (Springer Science & Business Media, 2009).

[2] A. M. Goossens, V. E. Calado, A. Barreiro, K. Watanabe, T. Taniguchi, and L. M. K. Vandersypen, Applied Physics Letters **100**, 073110 (2012).

[3] M. Field, C. G. Smith, M. Pepper, D. A. Ritchie, J. E. F. Frost, G. A. C. Jones, and D. G. Hasko, Physical Review Letters **70**, 1311 (1993).

[4] K. Todd, H.-T. Chou, S. Amasha, and D. Goldhaber-Gordon, Nano Letters **9**, 416 (2008).

[5] D. Bischoff, M. Eich, A. Varlet, P. Simonet, T. Ihn, and K. Ensslin, Physical Review B **91**, 115441 (2015).
